# Supplementary material for: Stochastic bubble dynamics in phase-separated scalar active matter
Source: arXiv:2501.11442 source file (2025-01-20)
Supplement: Supplementary file 1 [file Supplementary_Material.pdf]

# Stochastic bubble dynamics in phase-separated scalar active matter

Mingqi Yan, Erwin Frey, Marcus Müller and Stefan Klumpp

## Contents

|          |                                                                                          |           |
|----------|------------------------------------------------------------------------------------------|-----------|
| <b>1</b> | <b>Particle-based simulations</b>                                                        | <b>3</b>  |
| <b>2</b> | <b>Transformation of particle positions to particle density</b>                          | <b>4</b>  |
| <b>3</b> | <b>Identification and characterization of bubbles</b>                                    | <b>5</b>  |
| <b>4</b> | <b>Effective diffusion coefficient of bubbles</b>                                        | <b>9</b>  |
| 4.1      | Bubbles exhibit equal probability of movement towards the boundary or interior . . . . . | 10        |
| 4.2      | Bubble diffusion and interactions with droplet boundary . . . .                          | 11        |
| <b>5</b> | <b>Inference of drift and diffusion terms of the effective Langevin equation</b>         | <b>14</b> |
| 5.1      | Explanation for larger drift values in small bubbles . . . . .                           | 14        |
| 5.2      | Drift and diffusion of bubble areas measured at various time intervals . . . . .         | 15        |
| <b>6</b> | <b>Numerical determination of mean first passage time</b>                                | <b>17</b> |
| <b>7</b> | <b>Numerical Simulation of the Langevin Equation</b>                                     | <b>19</b> |
| <b>8</b> | <b>Langevin equation with sub-demographic noise</b>                                      | <b>20</b> |

|           |                                                              |           |
|-----------|--------------------------------------------------------------|-----------|
| <b>9</b>  | <b>Calculation of asphericity</b>                            | <b>24</b> |
| <b>10</b> | <b>The lattice gas model</b>                                 | <b>25</b> |
| 10.1      | Multiplicity of boundary sites . . . . .                     | 26        |
| 10.2      | Probabilities of adding or removing boundary sites . . . . . | 28        |
| 10.3      | Simulation parameters . . . . .                              | 28        |
| 10.4      | Dynamics of the lattice gas model . . . . .                  | 29        |
| <b>11</b> | <b>Supplemental movies</b>                                   | <b>31</b> |

# 1 Particle-based simulations

In particle-based simulations, we use the Euler-Maruyama scheme of discretization to model stochastic differential equations. For each particle, the values  $[x_t, y_t, \theta_t]$  are calculated from  $[x_{t-1}, y_{t-1}, \theta_{t-1}]$  using:

$$\begin{aligned}x_t &= x_{t-1} + v_0 \cos \theta_{t-1} \Delta t - \frac{1}{\gamma} \nabla_x U \Delta t + \sqrt{2D_T \Delta t} w_{x,t} \\y_t &= y_{t-1} + v_0 \sin \theta_{t-1} \Delta t - \frac{1}{\gamma} \nabla_y U \Delta t + \sqrt{2D_T \Delta t} w_{y,t} \\\theta_t &= \theta_{t-1} + \sqrt{2D_R \Delta t} w_{\theta,t}\end{aligned}$$

where  $w_{x,t}$ ,  $w_{y,t}$  and  $w_{\theta,t}$  are uncorrelated random numbers drawn from a Gaussian distribution with zero mean and unit standard deviation. The interaction  $U$  between particles is described by a WCA pair potential, as described in the main text. A neighbor list approach was implemented to optimize computational efficiency. The GPU code can be found in the Github repository<sup>\*</sup>.

---

<sup>\*</sup> <https://github.com/Mingqimingqi/Active-Brownian-Particle-Simulations>

## 2 Transformation of particle positions to particle density

To identify domains of liquid and vapor, we use a macroscopic (average) density field. To obtain this density field from the particle positions as given by the simulations, we average the microscopic number density,  $\hat{\rho}(\mathbf{r}) = \sum_{i=1}^N \delta(\mathbf{r} - \mathbf{r}_i)$  over a finite area,  $\xi^2$ . To this end, we divide the simulation box of geometry  $1085 \sigma \times 1085 \sigma$  into a square mesh with  $248 \times 248$  grid cells, i.e., each cell has a linear extent of  $\xi = 4.375 \sigma$ . We define the number of particles at a grid cell  $\mathbf{c}_j$  with  $j = 1, \dots, (L/\xi)^2$  by the convolution

$$m(\mathbf{c}_j) = \int d\mathbf{r} W(\mathbf{r}, \mathbf{c}_j) \hat{\rho}(\mathbf{r}) = \sum_{i=1}^N W(\mathbf{r}_i, \mathbf{c}_j). \quad (1)$$

The smoothed local number density is  $m(\mathbf{c}_j)/\xi^2$ . The assignment function  $W$  is designed to distribute the "mass" of each particle within a density mesh cell to its nearby grid points and obeys the normalization conditions

$$\sum_j W(\mathbf{c}_j, \mathbf{r}) = 1 \quad \forall \mathbf{r} \quad \text{and} \quad \int d^2\mathbf{r} W(\mathbf{c}_j, \mathbf{r}) = \xi^2 \quad \forall j. \quad (2)$$

This condition ensures that the contribution of each particle to all density mesh points sums to unity, regardless of the particle's position.

$\xi$  should be sufficiently large so that the probability distribution of the  $\xi^2$ -averaged densities has two distinct peaks, characterizing the liquid and vapor densities.  $\xi$  should be sufficiently small to resolve small vapor bubbles inside the liquid phase (and *vice versa*). The value  $\xi = 4.375 \sigma$  balances these two opposing requirements.

Specifically, we use a first-order assignment [1]

$$W(\mathbf{r}_i, \mathbf{c}_j) = w_x(|x_i - c_{j,x}|) w_y(|y_i - c_{j,y}|), \quad (3)$$

with

$$w_\alpha(|\Delta \mathbf{r}_\alpha|) = \begin{cases} 1 - \frac{|\Delta \mathbf{r}_\alpha|}{\xi} & \text{if } |\Delta \mathbf{r}_\alpha| \leq \xi \\ 0 & \text{otherwise} \end{cases}. \quad (4)$$

where  $c_{j,x}$  and  $c_{j,y}$  denote the Cartesian coordinates of the center of the grid cell  $\mathbf{c}_j$ . This results in a mapping of the discrete particle positions,  $\mathbf{r}_i$ ,  $i = 1, \dots, N$  onto a discrete set of numbers,  $m(\mathbf{c}_j)$ , of particle at grid cells  $\mathbf{c}_j$ ,  $j = 1, \dots, (L/\xi)^2$ , that depend continuously on the particle positions.

### 3 Identification and characterization of bubbles

To identify bubbles, we need to delineate vapor regions in the density field. Based on the density information obtained in the previous section, we can derive a bimodal distribution marking liquid and gas densities, as shown in Fig. S1. The system's density distribution exhibits two peaks corresponding to gas and liquid regions. We judiciously chose the system's average density ( $1024^2/L_x/L_y \times \xi^2 = 17.0489$ ) as the separation between the liquid and vapor phase, which nearly coincides with the minimum of the bimodal distribution. Generally, the average initial density determines the area fraction of liquid via the lever rule.

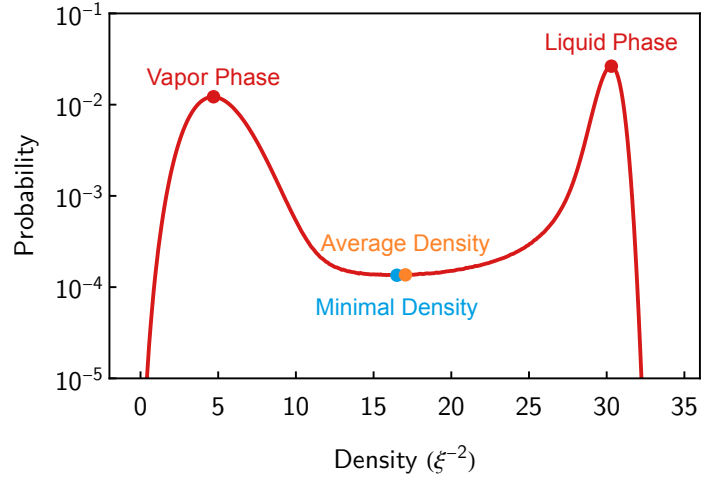

Figure S1. Probability distribution of density  $m(\mathbf{r})$  from particle-based simulations over the interval 4500 - 5000  $\tau$  (5001 time steps). The bimodal distribution exhibits a low-density peak corresponding to the vapor phase and a high-density peak representing the liquid phase, indicating phase separation. We use the average density to separate the liquid and vapor phases.

We can thus represent the density field using a binary color function, marking vapor regions ( $m(\mathbf{r}) \leq 17.0489 \xi^{-2}$ ) as white and liquid regions ( $m(\mathbf{r}) > 17.0489 \xi^{-2}$ ) as black. Fig. S2 illustrates both the original density plot and the

density plot after defining bubble boundaries. Subsequently, we use *Mathematica* to analyze bubble morphology based on this modified density plot.

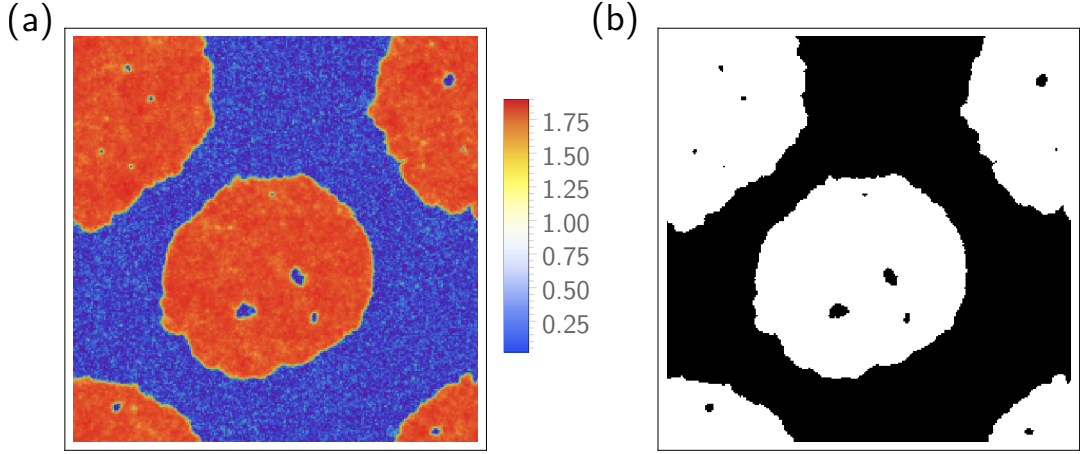

Figure S2. Comparison of the original density field  $m(\mathbf{r})/\bar{m}$  at  $t = 5000 \tau$  and the binary density used in analysis. The value 1 denotes the average density of the system. (a) Density field from particle-based simulations at  $t = 5000 \tau$ . (b) The same density field plotted using a binary color function, where values larger than 1 are white and smaller than 1 are black. This approach is valid as 1 approximately corresponds to the minimum point of the bimodal distribution.

**Analysis of bubble morphology.** We use the `ComponentMeasurements` function in *Mathematica* 14.0 to analyze bubble properties. This function takes an image as input (Fig. S2(b)), where one pixel corresponds to one density mesh ( $1 \xi^2$ ) and measures various bubble characteristics, including area, shape (pixel positions), center-of-mass location, and distance of center of mass to liquid boundary. To account for periodic boundary conditions, we prepared a 3 by 3 repetition of the original image and considered only non-repetitive complete liquid droplets. Table S1 presents an example output for the density

|                  | Bubble area ( $\xi^2$ ) | Bubble position ( $\xi$ ) | Bubble distance ( $\xi$ ) |
|------------------|-------------------------|---------------------------|---------------------------|
| Liquid droplet 1 | 4.25                    | 121.5, 151.25             | 9.25                      |
|                  | 64.25                   | 137.151, 101.119          | 44.4242                   |
|                  | 81.625                  | 105.275, 80.375           | 37.801                    |
|                  | 19.375                  | 147.237, 76.0263          | 19.2594                   |
| Liquid droplet 2 | 22.375                  | 274.591, 269.591          | 13.9094                   |
|                  | 18.5                    | 221.778, 254.944          | 16.1468                   |
|                  | 9.25                    | 281.722, 228.389          | 46.3268                   |
|                  | 42.875                  | 229.548, 220.881          | 39.8277                   |
|                  | 6                       | 295.5, 210                | 34.0037                   |
|                  | 2                       | 238.5, 179                | 33.6341                   |
|                  | 6.375                   | 265.667, 177.667          | 33.2374                   |
|                  | 1                       | 201.5, 171.5              | 1                         |
|                  | 1                       | 283.5, 168.5              | 14.7648                   |

Table S1. Bubble measurements for the density field at  $t = 5000 \tau$ . The table presents the original output for 13 bubbles (4 in droplet 1, 9 in the other droplet 2) from **Mathematica 14.0**. Columns show (1) bubble area, (2) center of mass coordinates ( $x, y$ ), and (3) distance from the center of mass to the nearest droplet boundary. All length measurements are in units of density mesh size ( $\xi$ ).

field at  $t = 5000 \tau$ . The minimal bubble area is 1 pixel, corresponding to  $1 \xi^2$  or  $4.375^2 \sigma^2$ .

**Tracking of bubble trajectories.** Having obtained bubble information at each time step, we proceeded to distinguish individual bubbles. This was accomplished by comparing the locations of bubble centers of mass between consecutive time steps. Bubbles with center-of-mass movements less than 5 pixels ( $5 \xi$ ) between time steps were identified as the same bubble. If no previous bubble was found within 5 pixels of the bubble's location, it was considered a new bubble. This threshold was chosen to maintain bubble identity even during merging events. As demonstrated in the supplementary video 4, this approach accurately constructs time series data of individual bubble behavior.

It should be noted that, when two bubbles merge, one bubble is considered to have disappeared one time step before the merging event, and the bubble that formed earlier inherits the bubble information. By selecting bubbles whose

area at the last time step is larger than 10 pixels but disappeared within the droplet (distance to boundary greater than 5 pixels), we found that merging events are rare, accounting for only 0.06 % of all bubbles. While this limitation exists, it does not impact our overall analysis due to the infrequency of such events.

## 4 Effective diffusion coefficient of bubbles

Using the methods described in Section 3, we obtained time series of bubble positions and areas. In Fig. S3(a) and (b), we present the raw data for the displacements of the bubble center in  $x$ - and  $y$ -direction, plotted against the bubble area,  $(A, dx)$  and  $(A, dy)$ , respectively. All data have a time step of  $\Delta t = 0.1 \tau$ , including 418,036 data points from bubbles with lifetimes exceeding one time step. For a given area  $A$ , both  $dx$  and  $dy$  follow a Gaussian distribution centered at zero, with their standard deviations decreasing as  $A$  increases.

From these displacements, we determine an effective short-time diffusion coefficient,  $D_{\text{eff}} = \frac{\langle \Delta L^2 \rangle}{2\Delta t}$  with  $\Delta L^2 = dx^2 + dy^2$ , which is shown in Fig. S3(c) as a function of the bubble radius  $r$ . This plot demonstrates that a larger radius corresponds to smaller effective diffusion coefficients, consistent with the trend of decreasing variance observed in Fig. S3(a) and (b). It is important to note that this is not the long-time diffusion constant, as the limit  $\Delta t \rightarrow \infty$  cannot be taken due to the finite lifetime of bubbles. Moreover, such a limit would be complicated by the non-constant area along the bubbles' trajectories.

This effective diffusion coefficient depends inversely on the bubble radius,  $r$  or, equivalently, on the length of the liquid-vapor interface,  $C \approx 2\pi r$  as shown in Fig. S3(c). This behavior can be understood through an analogy with a Rouse ring polymer model, where the bubble perimeter is divided into  $N_l \approx C/l$  independent segments of fixed length  $l$ . Each segment experiences thermal fluctuations, leading to a scaling relationship  $D_{\text{eff}} \sim \frac{1}{N_l} \sim \frac{1}{r}$ . In terms of the Rouse model, the effective friction is given by  $1/(rD_{\text{eff}})$  representing the resistance experienced by each segment. As shown in Fig. S3(d), this quantity is independent of the radius.

We also performed additional analyses by doubling  $\Delta t$  to  $0.2 \tau$ . In this case, the  $\langle \Delta L^2 \rangle$  term doubles, and consequently,  $D_{\text{eff}}$  remains unchanged. This consistency indicates that the effective friction we have defined is robust within the short-time regime we are investigating.

The measured diffusion coefficient can also be used to estimate the time a bubble takes to reach the domain boundary and merge with it. To reach the boundary, a bubble has to diffuse over a distance  $R$  that corresponds to the radius of the liquid domain. The time it takes to do so is then given by  $T_{\text{boundary}} \sim R^2/D_{\text{eff}}$ . The actual diffusion coefficient will change during that motion due to the size dependence, but we can obtain an order of magnitude

estimate with the largest measured values,  $D_{\text{eff}} \simeq 10^1 \sigma^2/\tau$ . Combining this with a liquid domain size of approximately a quarter of the simulation box size,  $R \simeq 100 \sigma$ , we arrive at an estimate for  $T_{\text{boundary}}$  of  $10^3 \tau$ , considerably longer than the typical bubble lifetimes we measured ( $\sim 10^0 \tau$ ).

#### 4.1 Bubbles exhibit equal probability of movement towards the boundary or interior

In the previous section, we have shown that the motion of bubbles is random (Fig. S3). As an additional test of whether the bubbles move towards the boundary of the liquid domain as in active model B+ [2], we determined the change in distance to the domain boundary over the lifetime of a bubble. Using the `Nearest` function in `Mathematica` 14.0, we determined the distance from each bubble's center of mass to the nearest liquid boundary at every time step. By comparing this distance at the first and last time step of each bubble's time series, we can assess whether bubbles have a tendency to move toward the liquid boundary. Fig. S4 presents a histogram of these distance changes for all bubbles. The data indicate that bubbles show no net flux towards the boundary, exhibiting an equal probability of moving towards the boundary (negative change) or the interior (positive change).

Based on the analysis in the previous section, we conclude that the center of mass of the bubble undergoes Brownian motion in two dimensions. Assuming a bubble has a fixed diffusion coefficient  $D$  and lifetime  $t$ , the displacement vector follows a Gaussian distribution, with mean 0 and variance  $2Dt$  for each direction. When converting to polar coordinates, the distribution of the magnitude of the center-of-mass displacement  $s = |\mathbf{s}|$  incorporates the phase-space factor  $2\pi s$ , resulting in

$$p(s, t) = \frac{s}{2Dt} \exp\left(-\frac{s^2}{4Dt}\right). \quad (5)$$

While an analytical solution for the bubble lifetime distribution remains elusive, we can empirically fit the lifetime distribution with  $P(t) = 0.188/(t^{1.25} + 0.118t^{2.5})$ , as shown in Fig. S5(a). Therefore, the probability distribution function of the bubble's center-of-mass displacement  $s$  is given by

$$p(s) = \int_0^\infty \frac{s}{2Dt} \exp\left(-\frac{s^2}{4Dt}\right) \cdot \frac{0.188}{t^{1.25} + 0.118t^{2.5}} dt. \quad (6)$$

As mentioned on page 2 of the main text, the mean area is  $284 \sigma^2$ . From Fig. S3(c), the effective diffusion constant is determined to be  $D_{\text{eff}} = 8 \sigma^2/\tau$ . Using this diffusion constant, we derived the theoretical distribution of the absolute center-of-mass displacement. The agreement between the theoretical predictions and simulation data in Fig. S5(b) suggests that the bubble motion can be well modeled as a random walk with a size-independent diffusion coefficient in the liquid phase.

## 4.2 Bubble diffusion and interactions with droplet boundary

If we weight the diffusion coefficients shown in Fig. S3(c) by the probability distribution of bubble areas, we obtain an average diffusion coefficient of  $16 \sigma^2/\tau$ . Given the mean bubble lifetime of  $1.49 \tau$ , the typical diffusion distance is approximately  $7 \sigma$ . With the chosen average density, the system contains almost equal areas of liquid and vapor phases. Assuming two droplets, the drop radius is  $R_d = \frac{L}{2\sqrt{\pi}} \approx 306 \sigma$ . Bubbles that are born within a distance  $\Delta R \approx 7 \sigma$  away from the liquid-vapor interface are potentially affected by the boundary. This amounts to a fraction of  $1 - (1 - \Delta R/R_d)^2 \approx 4.5\%$  of the total liquid area or  $4.5\%$  of all bubbles since born locations of bubbles are random. This agrees with our observation in the main text that only  $3\%$  of bubbles obviously interact with the liquid-vapor boundary.  $3\%$  was obtained by selecting those bubbles whose area at the last time step is larger than  $5 \xi^2$ .

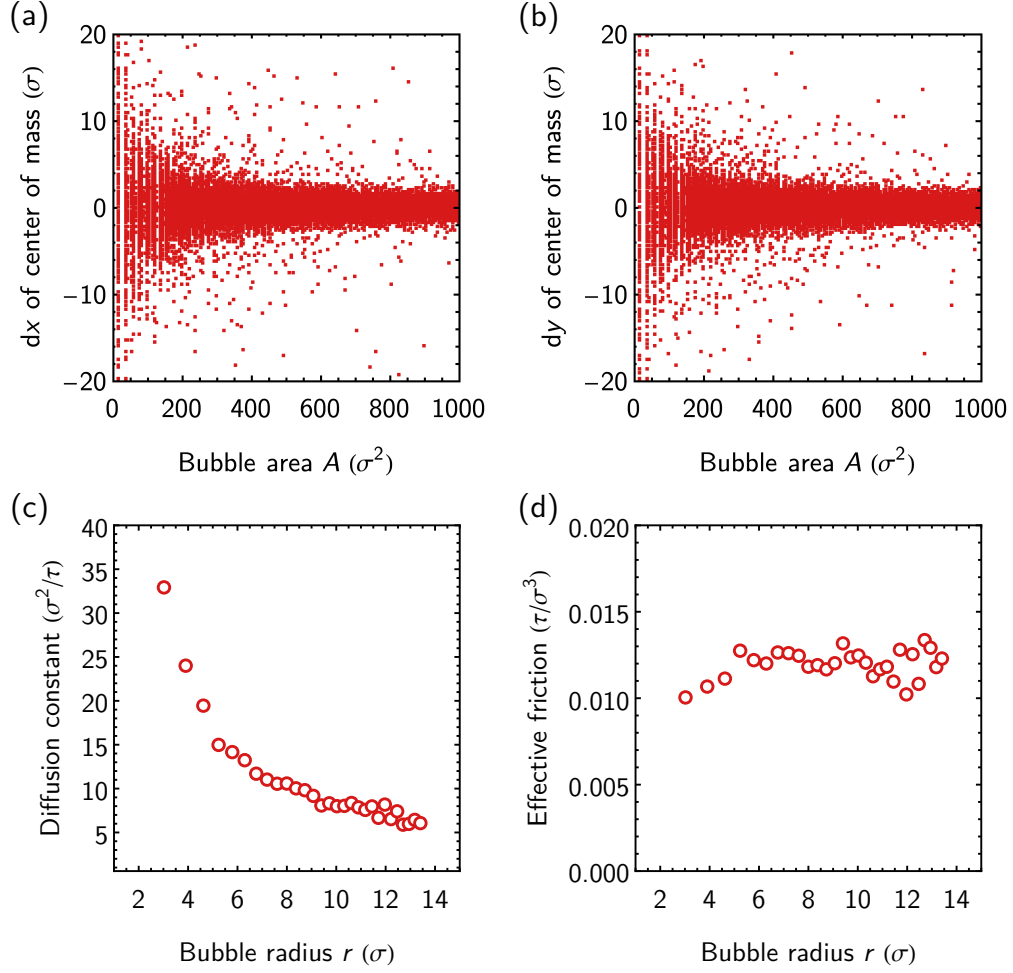

Figure S3. Relationship between short-time bubble diffusion constant and size. (a) Original data points of  $(A, dx)$  for all bubbles with lifetimes exceeding one time step. This graph includes 418,036 data points. All data in this figure are based on a time step of  $\Delta t = 0.1 \tau$ . (b) Similar plot for  $(A, dy)$ . (c) Relationship between effective diffusion coefficient  $D_{\text{eff}}$  and bubble radius  $r$ . (d) Relationship between effective friction  $1/(rD_{\text{eff}})$  and bubble radius  $r$ .

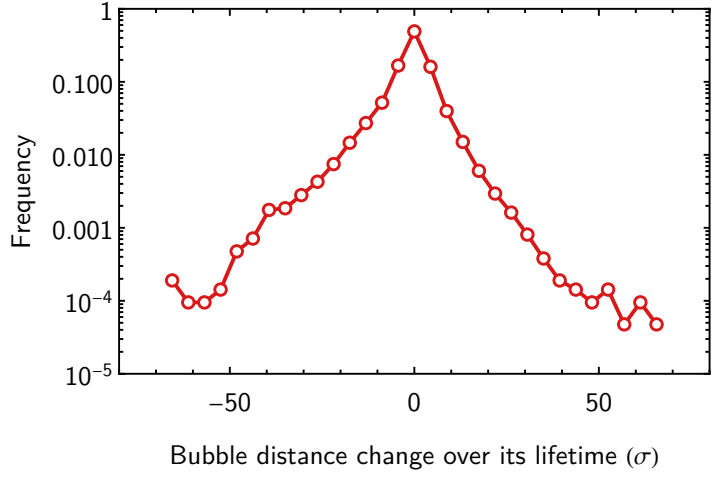

Figure S4. Histogram of distance changes relative to the boundary for all observed bubbles during their lifetime.

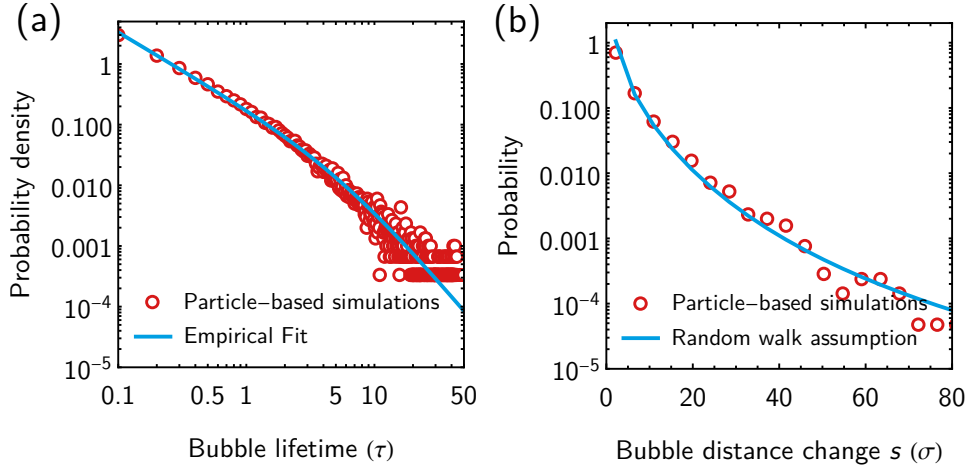

Figure S5. (a) Probability distribution of bubble lifetimes obtained from particle-based simulations (circles) with corresponding empirical fit  $P(t) = 0.188/(t^{1.25} + 0.118t^{2.5})$  (solid line). (b) Probability of the absolute center of mass displacement showing the comparison between particle-based simulations (circles) and theoretical predictions based on the random walk model (solid line).

## 5 Inference of drift and diffusion terms of the effective Langevin equation

### 5.1 Explanation for larger drift values in small bubbles

In Fig. 2(b) of the main text, we observed that the drift term in the Langevin equation inferred from the particle-based simulations was constant except for the first two data points. The deviation at small areas stems from the physical impossibility of certain  $dA$  values, which would result in negative areas, as shown in Fig. 2(a). Here, we provide an additional numerical demonstration to support this explanation.

To that end, we numerically generated data as in Fig. 2(b), based on the Langevin equation. We generated area changes  $dA$  by integrating the Langevin equation over a time step  $\Delta t$ , excluding all data points where the final area would be below the minimal resolution ( $1 \xi^2$  as described in Section 2 of this Supplementary Information), the smallest positive area that is detected in the particle-based simulations. The initial area values are drawn from the area distribution given by the analytical solution of the Fokker-Planck equation.

The specific numerical simulation procedure is as follows:

1. Select an area value from the analytical solution of the area distribution.
2. Generate an area change based on the stochastic term of the Langevin equation with  $\Delta t = 0.1 \tau$ .
3. If the new area after adding the area change is smaller than the resolution, we discard this operation; otherwise, we retain it.
4. Repeat steps 1-3 until 1 million valid  $(A, dA)$  pairs are obtained.
5. Calculate the average  $dA$  for each unique  $A$  value.

Fig. S6 shows that the data generated in this way closely aligns with the results from particle-based simulations. This result (and likewise the observation that the deviation from a constant is more pronounced for larger time steps, as shown in the following section and Fig. S7) provides further support for our interpretation that the observed deviation from a constant drift term for small areas does not reflect an actual increase of the drift, but rather unavoidable limitations in sampling area changes over a finite time step.

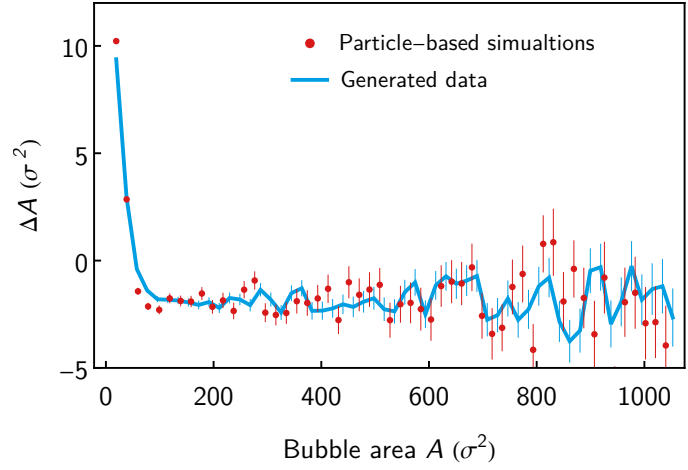

Figure S6. Comparison between numerically generated mean area change (blue solid line) and particle-based simulation (red cycles) for  $\Delta t = 0.1 \tau$ . Error bars represent standard deviations scaled by the square root of the sample size for each bubble area, reflecting the standard error.

## 5.2 Drift and diffusion of bubble areas measured at various time intervals

To test the validity of our Langevin equation, we examined how the choice of time increment  $\Delta t$  affects the inferred drift and diffusion terms. We compared the average bubble area shrinkage rate  $\nu$  and bubble area fluctuation parameter  $\Gamma$  for different choices of  $\Delta t$ . As shown in Fig. S7, both  $\nu$  and  $\Gamma$  remain constant across different  $\Delta t$  values, confirming the validity of the Langevin description. We also checked that the third and fourth moments of the area change are effectively zero, scaling super-linearly with  $\Delta t$ , as shown in Fig. S8.

When fitting  $\nu$  and  $\Gamma$ , we excluded the first two, three, and six data points for time steps  $\Delta t = 0.1 \tau$ ,  $0.2 \tau$ , and  $0.5 \tau$ , respectively, from the least-squares analysis. For these data points, the drift values are increased due to the missing area changes that would result in negative area values, as discussed in the previous section.

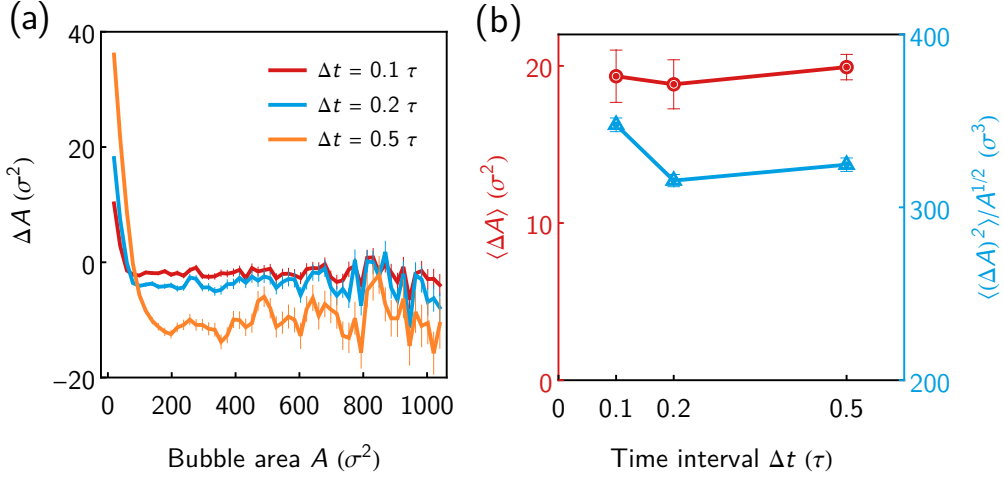

Figure S7. First and second moments of average bubble behavior. (a) Average change in bubble area  $\Delta A$ , measured for three different time increments  $\Delta t$ . (b) Average bubble shrinkage rate,  $\nu$  (red) and noise strength of bubble evolution,  $\Gamma$  (blue), plotted as a function of  $\Delta t$ . Both  $\nu$  and  $\Gamma$  are independent of  $\Delta t$ .

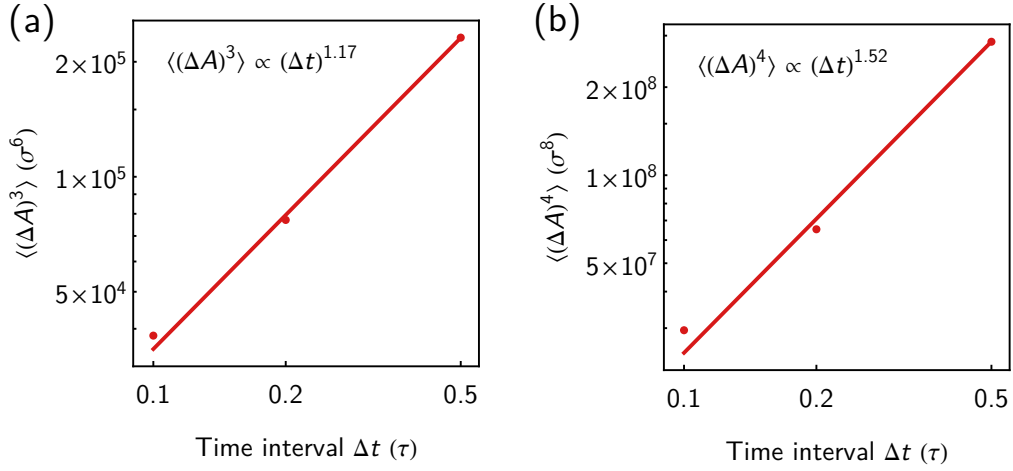

Figure S8. Mean third and fourth moments for bubble areas between 0 and  $1000 \sigma^2$  as a function of time interval  $\Delta t$ . They both scale super-linearly as a function of time increments. (a) Mean third moments. (b) Mean fourth moments.

## 6 Numerical determination of mean first passage time

First passage times for the vanishing of bubbles are determined from the bubble-area time series. Table S2 demonstrates this conversion for an example. The first column indicates the time step (with intervals of  $0.1 \tau$ , corresponding to the recording interval of particle-based simulations). The second column displays the bubble's area at each time step. The third column shows the corresponding pair of initial area and first passage time until the bubble dissolves, as given by the area at that time point and the steps taken until bubble dissolution. We exclude data from the final time step, as the bubble dissipated faster than our temporal resolution of  $0.1 \tau$ . By averaging first passage times with identical initial areas, we obtain the mean first passage time as a function of initial area, as presented in Fig. 3(b) of the main text.

Fig. S9 illustrates the conditional probability distribution of first passage times for given initial areas. As mentioned in the main text, for a given initial area, the distribution of first passage times follows an inverse Gaussian distribution. We also indicate the mean and mode of each inverse Gaussian distribution on the plot. The mean corresponds to the mean first passage time shown in Fig. 3(b) of the main text. The mode almost corresponds to the darkest point in each column for a given initial area.

|        | Area  | First passage time |
|--------|-------|--------------------|
| Step 1 | 3.125 | (3.125, 0.5)       |
| Step 2 | 4     | (4, 0.4)           |
| Step 3 | 3.125 | (3.125, 0.3)       |
| Step 4 | 3.125 | (3.125, 0.2)       |
| Step 5 | 2     | (2, 0.1)           |
| Step 6 | 1     | Will not be used   |

Table S2. Time series data of bubble area and derived first passage time for the first observed bubble. Time resolution is  $0.1 \tau$ .

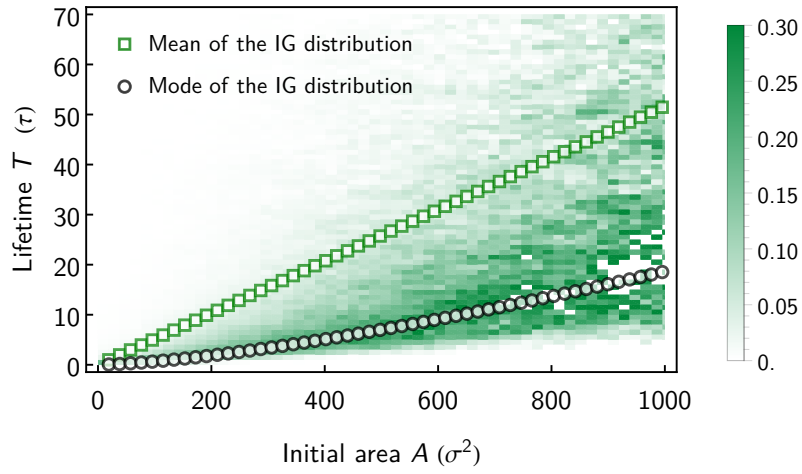

Figure S9. Lifetime distribution of bubbles for given initial areas. Green boxes indicate the mean first passage time (mean of the inverse Gaussian distribution), and black circles show the mode of each distribution.

## 7 Numerical Simulation of the Langevin Equation

In our Langevin equation simulations, we initialize the bubble area at the minimal size of our resolution ( $1 \xi^2 \approx 19.14 \sigma^2$ , refer to Section 2 of this Supplementary Information). At each time step, we update the bubble area according to the Euler-Maruyama discretization of the Langevin equation, with the diffusion term calculated from the area of the previous time step (Itô interpretation). We evaluate the bubble areas at each output step ( $\Delta t = 0.1 \tau$ ). If an area falls below the minimum resolution, we terminate its evolution and exclude its value for that last time step. Fig. S10 illustrates three sample trajectories. To ensure an accurate representation of the Langevin equation behavior, the data presented in the main text are derived from simulations of 1 million bubbles.

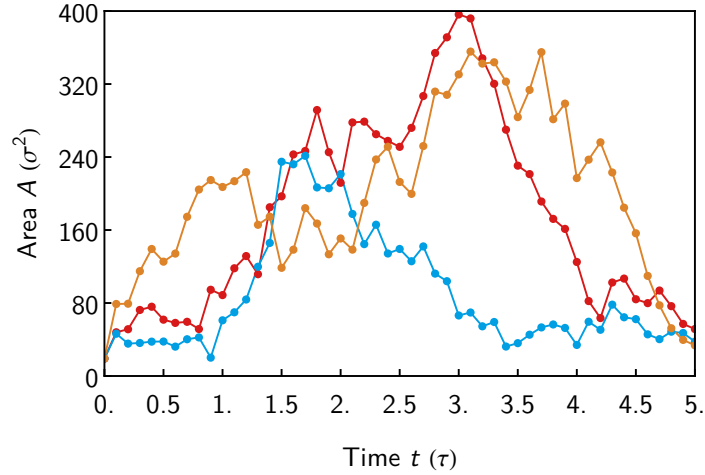

Figure S10. Time series of bubble areas for three simulations with time step  $dT = 10^{-5} \tau$ . We selected the first three simulations with lifetimes of  $5.0 \tau$  for visualization.

## 8 Langevin equation with sub-demographic noise

In the main text, we have investigated the stochastic dynamics of bubble area and found that the lowest moments of the incremental area change are given by

$$\langle \Delta A \rangle = -\nu \Delta t + o(\Delta t), \quad (7a)$$

$$\langle \Delta A^2 \rangle = 2\Gamma \sqrt{A} \Delta t + o(\Delta t). \quad (7b)$$

Assuming that the higher order moments are  $o(\Delta t)$  as indicated by Figure S8, this implies that the stochastic dynamics of the bubble area are given by the Fokker-Planck equation (FPE),

$$\partial_t p(A, t) = \partial_A [\nu p(A, t)] + \partial_A^2 [\Gamma \sqrt{A} p(A, t)], \quad (8)$$

where  $p(A, t)$  denotes the probability density for the bubble area at time  $t$ ; more precisely, the conditional probability density conditioned on the bubble area being  $A_0$  at time  $t = 0$ . This FPE with a state-dependent second moment is equivalent to a Langevin equation for the stochastic variable  $A_t$  in Itô interpretation

$$dA_t = -\nu dt + \sqrt{2\Gamma} A_t^{1/4} dW_t, \quad (9)$$

where  $dW_t$  denotes statistically independent stochastic increments with a Gaussian distribution of zero mean and unit variance.

This type of Langevin equation belongs to a broader class of stochastic processes with *sub-demographic multiplicative noise*

$$dA_t = -\nu dt + \sqrt{2\Gamma A_t^\alpha} dW_t. \quad (10)$$

The exponent  $\alpha$  ranges from 0 to 1, with  $\alpha = 0$  representing Brownian noise and  $\alpha = 1$  representing demographic noise. Specifically, when  $\alpha = 0$ , it corresponds to the classical problem of a Brownian particle in a gravitational field, where  $A$  denotes the vertical position of the particle. The case  $\alpha = 1$  represents a birth-death process characterized by equal birth and death rates, emigration at a rate  $\nu$ , and demographic noise arising from the inherent randomness of the birth and death events; now  $A$  indicates the number of individuals.

**Stationary state.** The stationary state of the above Fokker-Planck equation is determined by the condition that the probability current  $J$  is constant:

$$J = \nu p_{\text{eq}}(A) + \Gamma \partial_A [A^\alpha p_{\text{eq}}(A)]. \quad (11)$$

We are interested in the dynamics of an ensemble of bubbles. These bubbles are created at  $A = 0$  by nucleation events and then follow the dynamics described by the above Langevin equation (or its equivalent Fokker-Planck equation). Under this stochastic dynamics each individual bubble will eventually shrink to area zero and be absorbed at the boundary  $A = 0$ . For the system to be at a steady state the nucleation current and the absorption current must balance such that the net probability current equals zero. This corresponds to a Fokker-Planck equation with a reflective boundary condition at  $A = 0$ .

Then, defining  $\tilde{p}_{\text{eq}}(A) := A^\alpha p_{\text{eq}}(A)$  and using separation of variables one finds

$$\ln \tilde{p}_{\text{eq}}(A) = C - \frac{\nu}{\Gamma} \frac{A^{1-\alpha}}{1-\alpha}, \quad (12)$$

and hence

$$p_{\text{eq}}(A) = \frac{C}{A^\alpha} \exp \left[ -\frac{\nu}{\Gamma} \frac{A^{1-\alpha}}{1-\alpha} \right], \quad (13)$$

where  $C$  is an integration constant. In the limit  $\alpha = 0$ , this expression reduces to the barometric height formula  $p_{\text{eq}}(A) \sim \exp[-\nu A/\Gamma]$ . In the regime of sub-demographic noise, where  $\alpha < 1$ , the probability density remains normalizable, and a nontrivial steady state exists. However, for demographic noise,  $\alpha = 1$ , the probability distribution is no longer normalizable and steady states do not exist. Note also, that in the absence of drift the steady state does not exist either; the process does not become stationary for purely diffusive processes.

**Mean first passage time.** The mean first passage time  $T(A)$  can be obtained from [3]

$$-1 = -\nu \partial_A T(A) + \Gamma A^\alpha \partial_A^2 T(A). \quad (14)$$

It is an inhomogeneous parabolic differential equation, which for an absorbing boundary at  $A = 0$  (by standard methods) is solved by

$$T(A) = \int_0^A dx \frac{1}{\omega(x)} \int_x^\infty dy \frac{\omega(y)}{\Gamma y^\alpha} \quad (15)$$

with

$$\omega(x) = \exp \left[ \int_0^x dy \frac{\nu}{\Gamma y^\alpha} \right] = \exp \left[ -\frac{\nu}{\Gamma} \frac{x^{1-\alpha}}{1-\alpha} \right]. \quad (16)$$

Noting that  $\omega(x) \propto x^\alpha p_{\text{eq}}(x)$  this can also be written as

$$T(A) = \frac{1}{\Gamma} \int_0^A dx \frac{1}{x^\alpha p_{\text{eq}}(x)} \int_x^\infty dy p_{\text{eq}}(y) \quad (17)$$

Substituting  $z = y^{1-\alpha}$ , one obtains

$$\begin{aligned} \int_x^\infty dy p_{\text{eq}}(y) &= \int_x^\infty dy \frac{C}{y^\alpha} \exp \left[ -\frac{\nu}{\Gamma} \frac{y^{1-\alpha}}{1-\alpha} \right] \\ &= \frac{C}{1-\alpha} \int_{x^{1-\alpha}}^\infty dz \exp \left[ -\frac{\nu}{\Gamma} \frac{z}{1-\alpha} \right] \\ &= \frac{\nu}{\Gamma} C \exp \left[ -\frac{\nu}{\Gamma} \frac{x^{1-\alpha}}{1-\alpha} \right] \\ &= \frac{\nu}{\Gamma} x^\alpha p_{\text{eq}}(x). \end{aligned}$$

Hence, independent of the value of  $\alpha$  one obtains (for an absorbing boundary condition at  $A = 0$ ) that the mean first passage time is given by

$$T(A) = \frac{1}{\nu} A, \quad (18)$$

which is independent of the value of  $\alpha$ ; the results also matches the known result for a linear death process where the noise is demographic ( $\alpha = 1$ ).

It is interesting to ask how the mean extinction time depends on the average area (and not the actual area). The average area of a bubble, given by

$$\langle A \rangle = \int_0^\infty dx x p_{\text{eq}}(x), \quad (19)$$

scales as (with some numerical prefactor)  $\langle A \rangle \propto (\nu/\Gamma)^{1/(\alpha-1)}$ , such that the mean extinction time averaged over all bubble areas scales as

$$\langle T \rangle \propto \frac{1}{\Gamma} \langle A \rangle^{2-\alpha}. \quad (20)$$

For the special case  $\alpha = 1/2$  this gives

$$\langle T \rangle \propto \frac{1}{\Gamma} \langle A \rangle^{3/2}. \quad (21)$$

**General class of Langevin equations with subdemographic noise.** The results obtained above suggest to introduce a general class of Langevin equations with subdemographic noise by

$$dA_t = -\nu A_t^\beta dt + \sqrt{2\Gamma A_t^\alpha} dW_t. \quad (22)$$

Using the associated Fokker-Planck equation one finds for the steady state distribution

$$p_{\text{eq}}(A) \propto \frac{1}{A^\alpha} \exp \left[ -\frac{\nu}{\Gamma} \frac{A^{1+\beta-\alpha}}{1+\beta-\alpha} \right]. \quad (23)$$

The corresponding expressions for the first passage times can be obtained following a similar line of arguments as above.

If one were to cast this equation into pseudo-Onsager form, it would read

$$dA_t = -M(A_t) \partial_A F(A_t) dt + \sqrt{2M(A_t)} dW_t. \quad (24)$$

with  $M(A_t) = \Gamma A_t^\alpha$ , and the exponent  $\beta$  given by the form of the (pseudo-) free energy  $F(A)$ . Say, we assume that the free energy costs for creating a bubble scale as the perimeter of the bubble. Then, in  $d$  spatial dimensions we would have

$$F(A) = \chi A^{(d-1)/d}. \quad (25)$$

This gives  $\beta = \alpha - 1 + (d-1)/d$ . If in addition one assumes that the mobility also scales with the perimeter such that  $\alpha = (d-1)/d$ , then one gets  $\beta = 1 - 2/d$ ; for two dimensions one finds  $\beta = 0$  recovering the class studied above with a constant drift velocity  $\nu$ . For the  $d$ -dimensional case one finds that the steady state distribution is (for general values of  $\alpha$ ) given by

$$p_{\text{eq}} \propto \frac{C}{A^\alpha} \exp \left[ -\frac{d\nu}{(d-1)\Gamma} A^{(d-1)/d} \right] \propto \frac{C}{A^\alpha} \exp \left[ -F(A) \right]. \quad (26)$$

## 9 Calculation of asphericity

For a bubble with  $n$  elements, we have  $n$  pairs of coordinates representing the location of each element. All coordinates are expressed relative to the center of mass of the bubble. We then construct a matrix  $T$ , defined as:

$$T_{ij} = \frac{1}{n} \sum_{l=1}^n x_{il} x_{jl}, \quad (27)$$

where  $x_{il}$  denotes the  $i$ -th Cartesian component of the position vector of the  $l$ -th element. The eigenvalues of matrix  $T$  are denoted as  $\lambda_1$  and  $\lambda_2$ . We define the asphericity  $\Delta$  as the normalized difference of these two eigenvalues [4]:

$$\Delta = \frac{(\lambda_1 - \lambda_2)^2}{(\lambda_1 + \lambda_2)^2}. \quad (28)$$

The mean asphericity is obtained by averaging asphericity with the same areas. This formulation of asphericity provides a quantitative measure of the deviation from perfect spherical symmetry.

## 10 The lattice gas model

We propose a lattice gas model to reproduce the mean asphericity and area dynamics obtained from simulations of the particle-based model and the Langevin equation. The model represents a bubble as a collection of square elements in space. Based on random additions or removals of elements at the bubble boundary, we simulate the shape changes observed in particle-based simulations.

In this model, each lattice site represents a unit area of  $1 \xi^2$ , aligning with the density mesh size described in Section 2 of this Supplementary Information. The model evolves using the Gillespie algorithm, where each update involves either removing a boundary element or adding an element to the boundary. The total rate in the Gillespie algorithm consists of two parts, corresponding to the drift and diffusion terms in the Langevin equation. The drift rate is a constant value, while the diffusion rate is proportional to the perimeter of the bubble. Consequently, larger bubbles with greater perimeters experience more frequent addition or removal events at their boundaries.

In our simulations, the initial configuration is a single element, representing an area of  $1 \xi^2$ . We evolve the system until the area becomes less than  $1 \xi^2$ . The resulting data includes the update times of the lattice configuration and the position coordinates of the area elements, which are used to calculate asphericity.

Our model has three parameters: two rate parameters and one effective interaction parameter. The rate  $\alpha_1$  corresponds to the drift term, and the rate  $\alpha_2$  corresponds to the diffusion term. Additionally, the effective interaction  $\epsilon$  is used to determine the relative probabilities of different sites being selected in an addition or removal event. The algorithm proceeds as follows:

1. For a given bubble, determine the perimeter, defined as  $C = 2\sqrt{\pi N}$ , where  $N$  is the number of area elements.
2. Determine when the next event will happen based on the total rate  $R = \alpha_1 + \alpha_2 C$ . The time to the next event is given by  $t_{\text{next}} = \frac{1}{R} \log(1/r_1)$ , where  $r_1$  is a random number uniformly distributed between 0 and 1. Another uniformly distributed random number  $r_2$  ( $0 < r_2 < 1$ ) determines whether the event corresponds to a drift or diffusion event. If  $r_2 < \alpha_1/R$ , execute a removal event; otherwise, execute a diffusion event, where with equal probability (of  $1/2$ ) a boundary element is added or removed.

- a) For an adding event:
  - i. Identify all possible growth sites. These are the unoccupied nearest neighbors and next-nearest neighbors of all area elements.
  - ii. Assign multiplicities  $m_i$  to these possible growth sites  $i$  as follows: count the numbers of nearest neighbors (connected by one edge) and next-nearest neighbors (connected through a corner point) that are 'occupied', i.e., are part of the bubble; see section 10.1 for the definition of these multiplicities.
  - iii. Based on these multiplicities, calculate the probability  $p_i^{\text{add}}$  for adding an area element to the bubble boundary; see Section 10.2 for the definition of these probabilities.
  - iv. Select a position  $i$  to add an area element, based on the probabilities  $p_i^{\text{add}}$ .
- b) For a removal event:
  - i. Identify all boundary elements (i.e., bubble elements in contact with surrounding empty space).
  - ii. Calculate multiplicities  $m_i$  of boundary elements as if they were already removed, using the same rules defined above.
  - iii. Calculate probabilities  $p_i^{\text{remove}}$  based on the multiplicities, where  $p_i^{\text{remove}} = 1 - p_i^{\text{add}}$ .
  - iv. Select an area element at position  $i$  to be removed based on the calculated probabilities  $p_i^{\text{remove}}$ .

3. Go to step 1 as long as the number of elements is larger than 1.

## 10.1 Multiplicity of boundary sites

We illustrate the multiplicity calculation for a given site through three examples, illustrated in Fig. S11.

1. For a single-element bubble (Fig. S11(a)), there are 8 possible growth sites. For both nearest neighbors and next-nearest neighbors, the assigned multiplicity is 1, since they touch a *single* area element either through an edge or a corner, respectively.

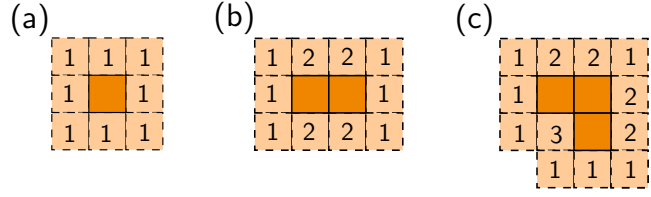

Figure S11. Multiplicity calculations for potential growth sites in different bubble configurations. (a) An initial seed with only one area element has 8 possible growth sites, each with multiplicity 1 for both nearest and next-nearest neighbors. (b) For two-element bubbles, growth sites exhibit multiplicities up to 2, arising from contacting one bubble element via an edge and another via a corner. (c) In a three-element triangular configuration, the highest multiplicity reaches 3 by contacting two bubble elements through edges and one via a corner.

2. For two-element bubbles (Fig. S11(b)), we again determine the multiplicities of the possible growth sites by counting the number of area elements they touch, either through an edge or a corner. Note that the multiplicity of 2 arises because those growth sites contact one area element of the bubble via an edge and another via a corner.
3. For a three-element triangle configuration (Fig. S11(b)), the multiplicities of the possible growth sites include a value of 3 for the area element that would complete the triangle configuration into a square. It arises because it touches two of the bubble's area elements by an edge and one by a corner. It is the highest multiplicity value possible for this configuration.

As illustrated in the examples above, calculating these multiplicities involves counting the area elements within the bubble that contact the tentative growth sites, either through an edge or a corner. For addition events, all existing area elements can potentially contribute. In contrast, for removal events, the multiplicity is determined under the assumption that the site in question has already been removed.

We have examined whether the assignment of these multiplicities can be simplified. Specifically, if contributions from next-nearest neighbors are ignored, the mean asphericity decreases more rapidly as bubbles grow larger.

## 10.2 Probabilities of adding or removing boundary sites

We assume that the probability of selecting a site  $i$  with multiplicity  $m_i$  for adding or removing an area element is given by a Boltzmann factor,

$$p_i^{\text{add}} = 1 - p_i^{\text{remove}} = \frac{e^{\epsilon m_i}}{Z}, \quad (29)$$

where  $\epsilon$  denotes the interaction scale and  $Z$  a normalization factor

$$Z = \sum_i e^{\epsilon m_i}. \quad (30)$$

with the sum running over all possible sites  $i$  for the current event.

## 10.3 Simulation parameters

The lattice gas model has three parameters: two rate parameters ( $\alpha_1$  and  $\alpha_2$ ) and an interaction parameter ( $\epsilon$ ).

First, we determine the rates  $\alpha_1$  and  $\alpha_2$  from the Langevin equation

$$dA_t = -\nu dt + \sqrt{2\Gamma} A_t^{1/4} dW_t. \quad (31)$$

In the lattice gas model, for a bubble containing  $N$  area elements, the transition rate to a bubble configuration with  $N + 1$  area elements is  $\alpha_2 C/2$ , where  $C$  represents the bubble's perimeter, assuming it is spherical. Conversely, the probability of transitioning to a bubble configuration with  $N - 1$  area elements reads  $\alpha_1 + \alpha_2 C/2$ . The expectation value for the change  $\Delta A$  in the bubble area resulting from these processes is  $\langle \Delta A \rangle = -\alpha_1$ . It corresponds to the drift term in the Langevin equation, thus giving  $\alpha_1 = \nu$ .

The second moment of  $\Delta A$  in the lattice gas model is  $\alpha_1 + \alpha_2 C$  and corresponds to the diffusion term  $2\Gamma\sqrt{A}$  in the Langevin equation. For a circular bubble, the perimeter is  $C = 2\sqrt{\pi A}$ . Ignoring the small value of  $\alpha_1$ , we identify  $\alpha_2 = \frac{\Gamma}{\sqrt{\pi}}$ .

In the main text, we used the particle diameter  $\sigma$  as unit of length, whereas the lattice gas model measures lengths in units of  $\xi = 4.375\sigma$ . Thus, we obtain

$$\alpha_1 = \nu = 19.2 \frac{\sigma^2}{\tau} \approx 1.01 \frac{\xi^2}{\tau} \quad (32)$$

$$\alpha_2 = \frac{\Gamma}{\sqrt{\pi}} = \frac{348 \frac{\sigma^3}{\tau}}{\sqrt{\pi}} = 2.34 \frac{\xi^3}{\tau} \quad (33)$$

The interaction  $\epsilon$  is determined to be 1.1 by comparing the mean asphericity of large bubbles with particle-based simulations. Note that only  $\epsilon$  influences the value of mean asphericity, and larger values of  $\epsilon$  result in smaller mean asphericity.

We generated 100,000 bubbles using the described algorithm and parameters and analyzed their asphericity (discussed in the main text) and dynamics (discussed in the next section).

## 10.4 Dynamics of the lattice gas model

The lattice gas model (with its parameters chosen as described above) not only characterizes the bubble shape (asphericity) but also captures key dynamical properties. As shown in Fig. S12(a) and (b), the model accurately reproduces lifetime and area distributions, showing the equivalence between the lattice gas model and the bubble evolution, as obtained from particle-based simulations.

Our findings indicate that random events at the bubble boundary determine bubble evolution, with event probabilities approximately proportional to the bubble's perimeter.

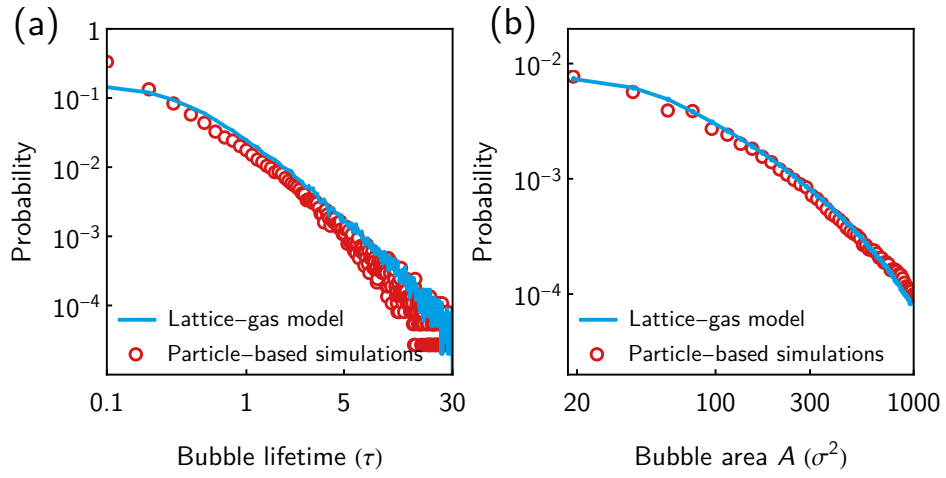

Figure S12. Comparison of bubble dynamics between particle-based simulations (open red circles) and the lattice gas model (blue solid lines). (a) Probability distribution of bubble lifetimes. (b) Probability distribution of bubble areas. The lattice gas model reproduces the essential statistical properties observed in the particle-based simulations.

## 11 Supplemental movies

We provide four supplementary videos to illustrate the main results of our study:

1. Video 1 shows the time evolution of the density from  $0 \tau$  to  $5000 \tau$  (units:  $1/\xi^2$ ).
2. Video 2 displays the evolution of the bubble depicted in Fig. 1(a), with the color scale normalized to the initial average density of  $17.0489 \, 1/\xi^2$ . This bubble is labeled ID 27620 in Video 4 (see SI Section 3 for details).
3. Video 3 illustrates the evolution of the bubble shown in Fig. 1(b), using the same color scale based on the initial average density of  $17.0489 \, 1/\xi^2$ . This bubble is labeled ID 25634 in Video 4 (see SI Section 3 for details).
4. Video 4 contains all bubbles analyzed in this study, highlighted in white and assigned unique IDs. For each bubble, the time step, lifetime, and area are indicated (see SI Section 3 for details).

## References

- [1] M. Müller, “Studying amphiphilic self-assembly with soft coarse-grained models”, [Journal of Statistical Physics](#) **145**, 967–1016 (2011).
- [2] E. Tjhung, C. Nardini, and M. E. Cates, “Cluster Phases and Bubbly Phase Separation in Active Fluids: Reversal of the Ostwald Process”, [Phys. Rev. X](#) **8**, 031080 (2018).
- [3] C. Gardiner, *Handbook of Stochastic Methods for Physics, Chemistry, and the Natural Sciences*, Springer complexity (Springer, 2004).
- [4] J. Rudnick and G. Gaspari, “The Shapes of Random Walks”, [Science](#) **237**, 384–389 (1987).
